# Supplementary material for: 3DP3: 3D Scene Perception via Probabilistic Programming
Source: arXiv:2111.00312 source file (2021-10-30)
Supplement: Supplementary file 1 [file appendix.tex]

\section{Appendix}

Optionally include extra information (complete proofs, additional experiments and plots) in the appendix.
This section will often be part of the supplemental material.
