# Supplementary material for: 3DP3: 3D Scene Perception via Probabilistic Programming
Source: arXiv:2111.00312 source file (2021-10-30)
Supplement: Supplementary file 3 [file full-page-figures.tex]

%\begin{figure}[ph!]
%	\centering
%	\includegraphics[width=0.9\textwidth]{paper_figures/full_page_v2.pdf}
%	\caption{Pose estimates of DenseFusion and 3DP3 on YCB scenes. YCB objects: 002\_master\_chef\_can, 003\_cracker\_box, 004\_sugar\_box, 005\_tomato\_soup\_can, 006\_mustard\_bottle, 007\_tuna\_fish\_can}
%	\label{fig:ycb_qual_1}
%\end{figure}

%\begin{figure}[ph!]
%	\centering
%	\includegraphics[width=0.9\textwidth]{paper_figures/full_page_tile_2.pdf}
%	\caption{Pose estimates of DenseFusion and 3DP3 on YCB scenes. YCB objects: 008\_pudding\_box, 009\_gelatin\_box, 010\_potted\_meat\_can, 011\_banana, 019\_pitcher\_base, 021\_bleach\_cleanser}
%	\label{fig:ycb_qual_2}
%\end{figure}
%
%\begin{figure}[ph!]
%	\centering
%	\includegraphics[width=0.9\textwidth]{paper_figures/full_page_tile_3.pdf}
%	\caption{Pose estimates of DenseFusion and 3DP3 on YCB scenes. YCB objects: 024\_bowl, 025\_mug, 035\_power\_drill, 036\_wood\_block, 037\_scissors, 040\_large\_marker}
%	\label{fig:ycb_qual_3}
%\end{figure}
%
%
%\begin{figure}[ph!]
%	\centering
%	\includegraphics[width=0.9\textwidth]{paper_figures/full_page_tile_4.pdf}
%	\caption{Pose estimates of DenseFusion and 3DP3 on YCB scenes. YCB objects: 051\_large\_clamp, 052\_extra\_large\_clamp, 061\_foam\_brick}
%	\label{fig:ycb_qual_4}
%\end{figure}
